# Supplementary material for: Lifetime of racetrack skyrmions
Source: arXiv:1706.07173 source file (2017-10-02)
Supplement: Supplementary file 1 [file supplementary_information.pdf]

## Supplementary Information for “Annihilation mechanisms and lifetime of racetrack skyrmions”

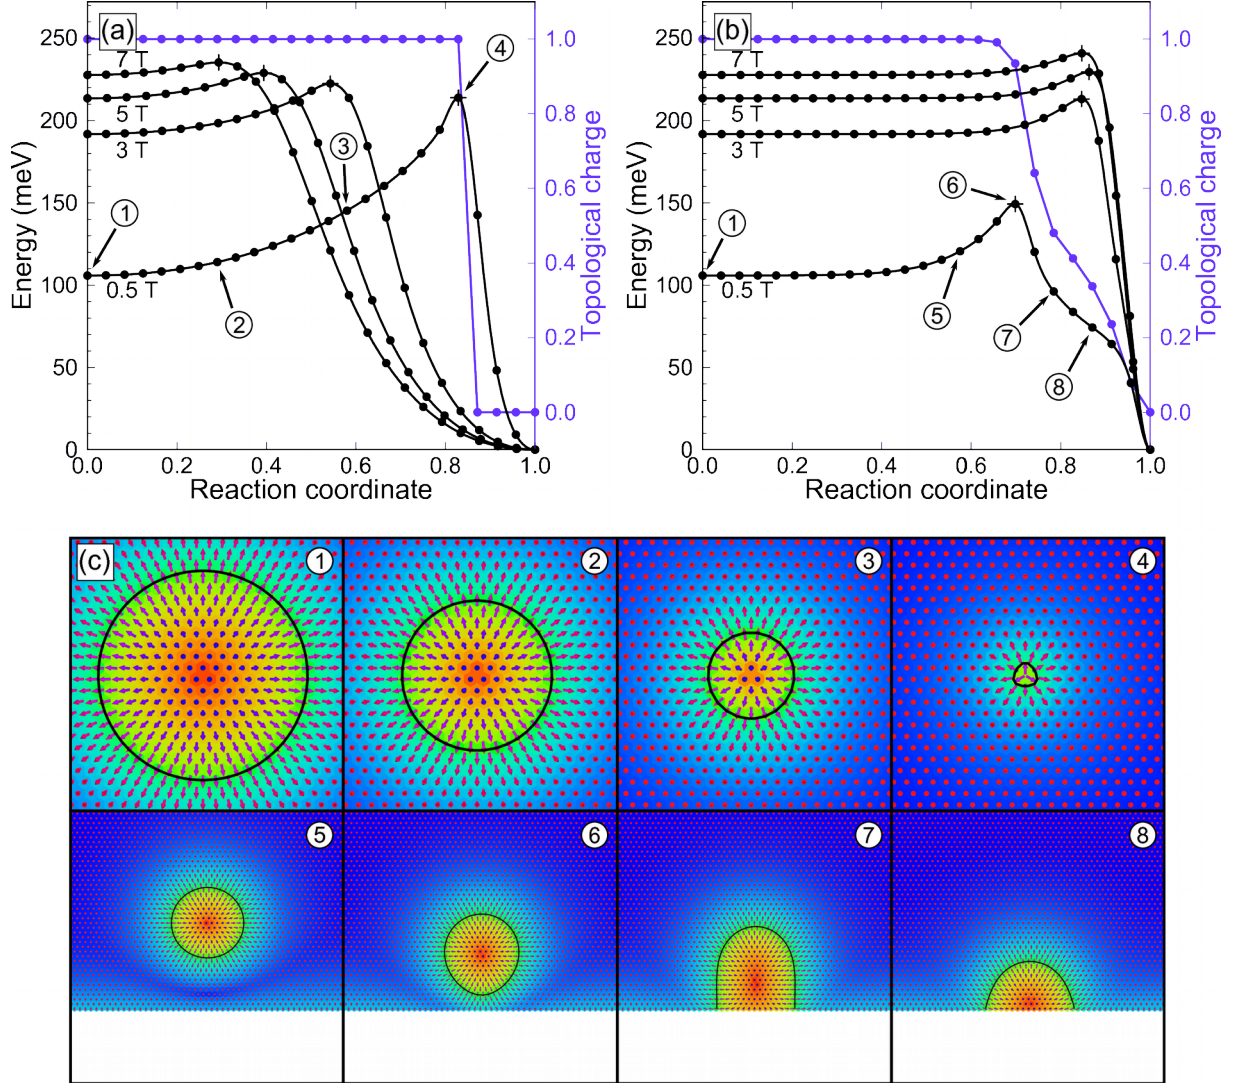

**Supplementary Figure 1 | Mechanisms of the skyrmion annihilation in a hcp-Pd/Fe racetrack on Ir(111).**

Energy variation along the minimum energy paths (MEPs) for radial collapse of the skyrmion at the interior of the strip (a) and escape of the skyrmion through the boundary (b), shown for four values of applied magnetic field. The filled circles show position of the intermediate states along the annihilation paths, while crosses indicate energy maxima along the MEPs. Variation of the topological charge along the MEPs is shown with a purple line for  $B = 0.5$  T. The reaction coordinate is defined as the normalized displacement along the MEP. Starting- and end-point of the reaction coordinate is the skyrmion and ferromagnetic state, respectively. The encircled numbers label the images for which spin configurations are shown in the lower panel (c). The background color indicates the value of the out-of-plane component of the magnetic vectors (red ↔ up, blue ↔ down). Black solid lines show the contour where the out-of-plane component of magnetization vanishes.

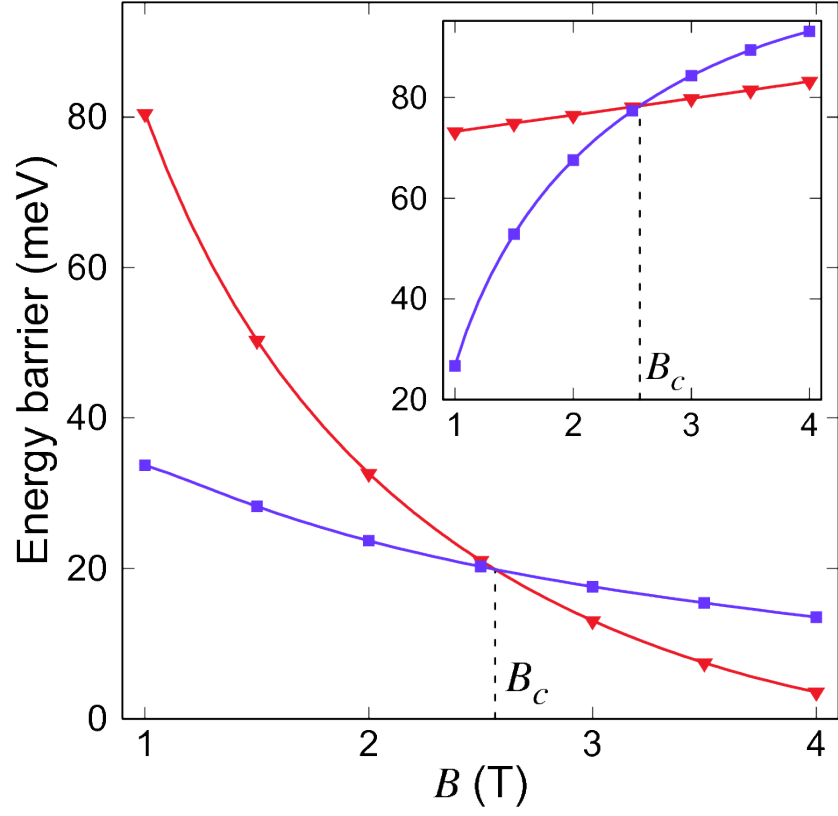

**Supplementary Figure 2 | Energy barriers for skyrmion annihilation in a Pd/Fe/Ir(111) racetrack described by the effective, nearest neighbor exchange model.** Energy barrier for the skyrmion annihilation and nucleation (inset) at the interior (red curve, triangles) and at the boundary (purple curve, squares) of the Pd/Fe strip as a function of applied field strength. The curves intersect at the crossover field,  $B_c$ . Parameters of the effective Hamiltonian are taken from Ref. [7] of the main text.

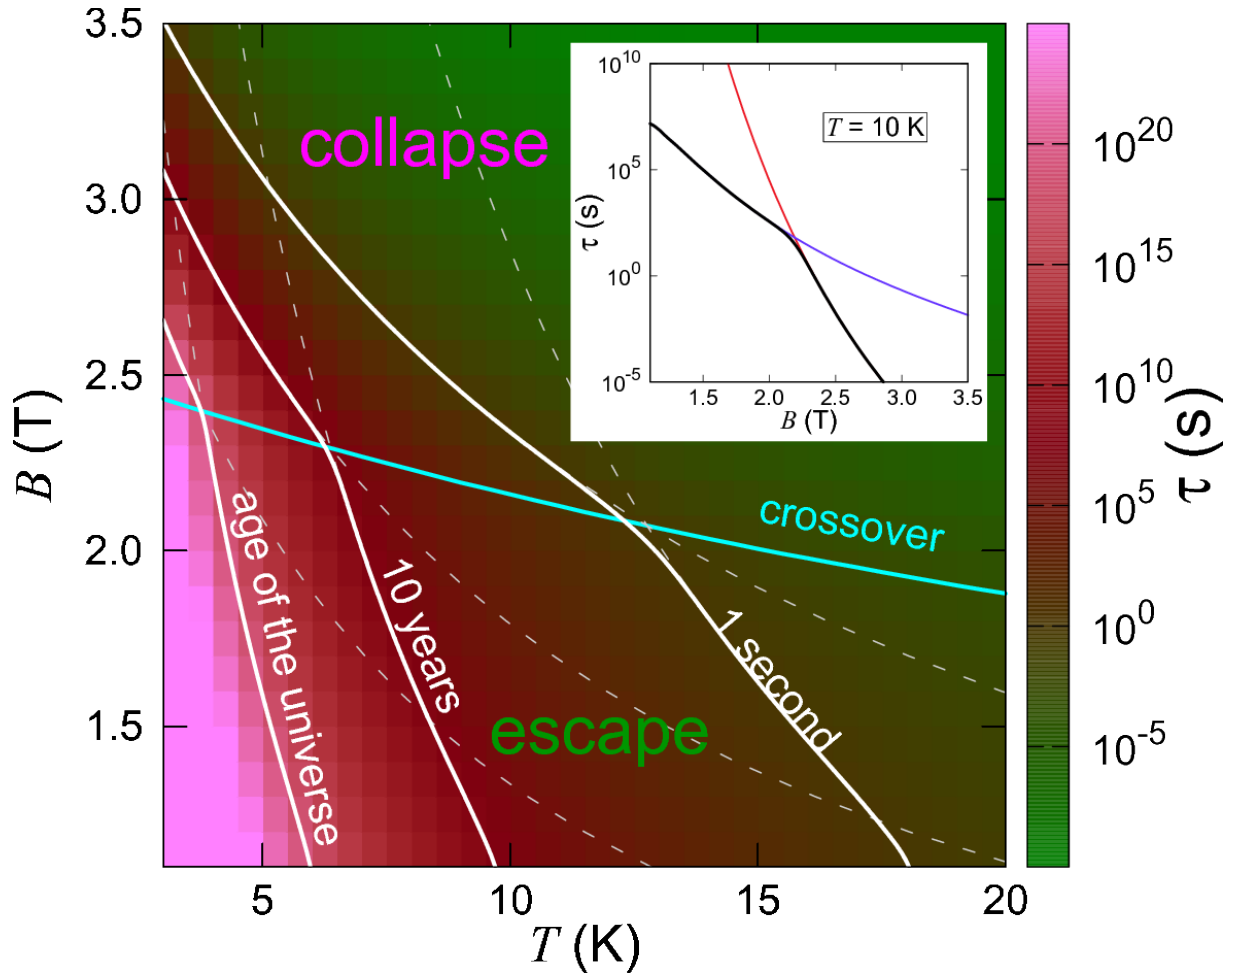

**Supplementary Figure 3 | Lifetime of a skyrmion in a Pd/Fe/Ir(111) racetrack described by the effective, nearest neighbor exchange model.** Contour plot of the calculated lifetime of an isolated skyrmion in a 23.5 nm wide strip as a function of applied magnetic field strength and temperature. White contour lines have a characteristic cusp due to the crossover indicated by the cyan line. White dashed lines indicate contours of the collapse and escape relaxation times. Inset shows the cut of the contour plot at  $T = 10$  K; in the insets, annihilation time due to collapse at the interior, escape through the boundary and total skyrmion lifetime are shown with red, purple and black curves, respectively. Parameters of the effective Hamiltonian are taken from Ref. [7] of the main text.
